# Supplementary material for: Topological Data Analysis for Unsupervised Feature Selection in Large Scale Spatial Omics Data Sets
Source: arXiv:2505.04360 ancillary file (2025-09-08)
Supplement: Supplementary file 1 [file supplementary_material.pdf]

# Supplementary Material

In this document we provide further methodological details, discussion and visualisations designed to supplement the main text. The material here is designed to be read in conjunction with the main paper, and we use the same terminology, and notation as defined therein.

## Supplementary Analysis

### Application of PersiST to MSI Data

Some differences in the MSI sample compared to the spatial transcriptomics samples necessitated some modifications to the default application of applied PersiST. These modifications highlight both some of the finer workings of PersiST, as well as some differences between spatial transcriptomics and MSI data. This exhibits some of the difficulties that can arise when translating a data analysis methodology from one spatial modality to another.

### Larger Sample Size Necessitates a Different Level of Smoothing

The first step PersiST takes is to smooth the input data, with a parameter  $m \in (0, 1)$  controlling the level of smoothing to apply. As  $m$  increases, the percentage of the tissue a spatial feature must take up in order to not be completely smoothed out increases. For the spatial transcriptomics samples, we found that  $m = 0.1$  struck a good balance between smoothing out noise, whilst retaining spatial features of interest. The MSI sample we analysed contained a significantly larger number of points where the intensity was measured, and we found that a lower value of  $m = 0.01$  struck the appropriate balance.

In general, the lower the proportion of the tissue sample one might expect a spatial feature to take up, the lower one should set  $m$ . This will depend on both the number of points and the spatial resolution of the sample.

### SVM Calling Complicated by Different CoSS-Rank Profile

For the spatial transcriptomics data sets, the vast majority of genes had very little spatial structure (and thus a very low CoSS), and the CoSS-rank plot possessed a very sharp elbow that enabled a sensible cutoff to be decided (figure 1d, supplementary figure 1c). For the MSI sample the CoSS-rank plot showed a gradual decline in the CoSS before a sharp drop off at the end (supplementary figure 1c). This complicated the process of making a binary call of spatial variability.

One possibility is that this CoSS-rank profile was driven by technical artefacts that affected a large proportion of the data set. For example, we observed that a large proportion of the metabolites displayed higher intensity and/or more spatial variation towards the top of the tissue sample (supplementary figure 1b). This effectively adds some spatial structure to all affected metabolites, but produces greater CoSS inflation for those affected metabolites with otherwise low spatial structure,

blunting the sharp elbow structure we see in the CoSS-rank plots for the spatial transcriptomics samples.

Alternatively, there may generally be a more gradual gradient of spatial structure in MSI datasets, lessening the distinction between spatially variable and not when making a binary call. Further work is needed on analysis with continuous spatial structure scores in the absence of a sharp ‘elbow’.

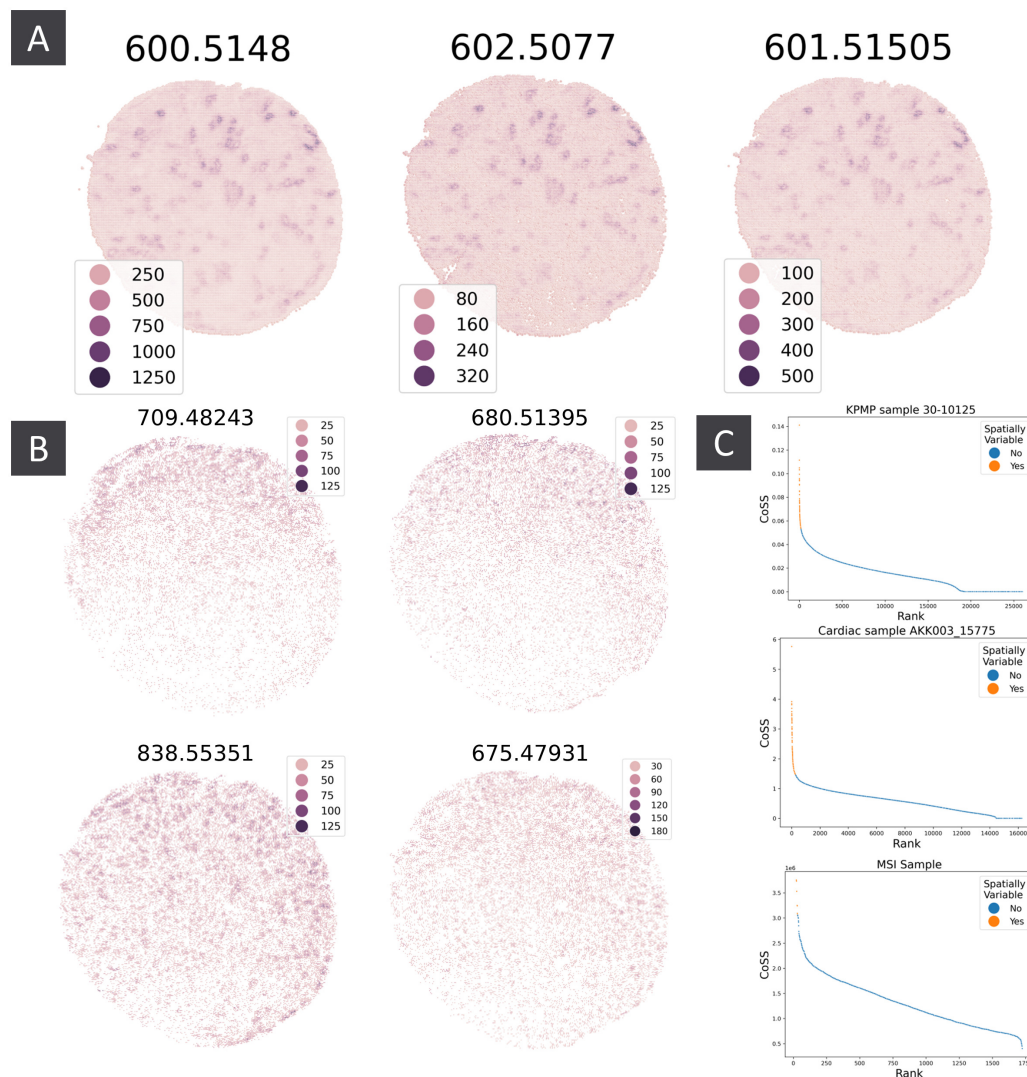

Supp Fig. 1: a) Co-localised metabolites of the same molecular species - a ceramide identified as Cer(36:1). b) Examples of metabolites with intensity biased towards the upper half of the sample. Many metabolites displayed patterns like this, and it is unclear whether this reflects genuine biology or sampling artefacts. c) CoSS-Rank plots for exemplar spatial transcriptomics samples from the kpmp and cardiac cohorts, and the MSI sample. The MSI plot displays a heavier “tail”, with a large proportion of metabolites displaying some spatial structure.

## Supplementary Methods

Here we give some further specifics on how PersiST computes CoSS for each gene.

### Aligning Well Co-Ordinates to a Network Structure

Given raw co-ordinate data for each well, PersiST automatically aligns the wells to a regular network of the type specified.

We determine wells  $i$  and  $j$  to be adjacent in this network if  $d_{ij} < Sd_{\min}$ , where  $d_{\min} = \min\{d_{ij}\}_{ij}$ , and  $S$  is a scaling factor dependent on the grid type ( $S = (1 + \sqrt{3})/2$  for a hexagonal grid, and  $S = (1 + \sqrt{2})/2$  for a square grid). This is equivalent to considering wells to be adjacent if they are separated by a distance less than halfway between the minimal observed distance between wells, and the second nearest neighbour distance in a regular network where the minimum observed inter-well distance is the well separation.(supplementary figure 2a).

We use  $Sd_{\min}$  as a cutoff rather than just  $d_{\min}$  to allow for slight mis-specification of the well co-ordinates, or slight misalignment of the wells.

### Artefact Detection

Consider the gene expression pattern shown in supplementary figure 2c. Taken as a genuine expression pattern, this is highly spatially heterogeneous. However, it is also possible that such an expression pattern could be the result of technical artefacts. It is typically not possible to determine which is the case from the data alone, so instead PersiST flags such genes as “possible artefacts”, and leaves it to the practitioner to decide how to proceed. Here we outline and motivate how this is done.

Such genes are characterised by having the vast majority of their spatial structure explained by a single feature. In the 0 dimensional barcode, this looks like one very long bar against a collection of significantly smaller ones (supplementary figure 2d). Thus to detect possible artefacts, we look at the ratio of the longest bar to the sum of all lengths of bars. In mathematical language, this is the ratio of the  $L^\infty$  to the  $L^0$  norm of the barcode.

By default, PersiST flags any gene for which this ratio exceeds 0.9 as a possible artefact. In the authors’ experience this strikes the right balance between identifying technical artefacts, but not ruling out genuine patterns of spatial variability. PersiST also contains the option for the practitioner to set this threshold themselves, and PersiST outputs the ratios for downstream analysis if desired.

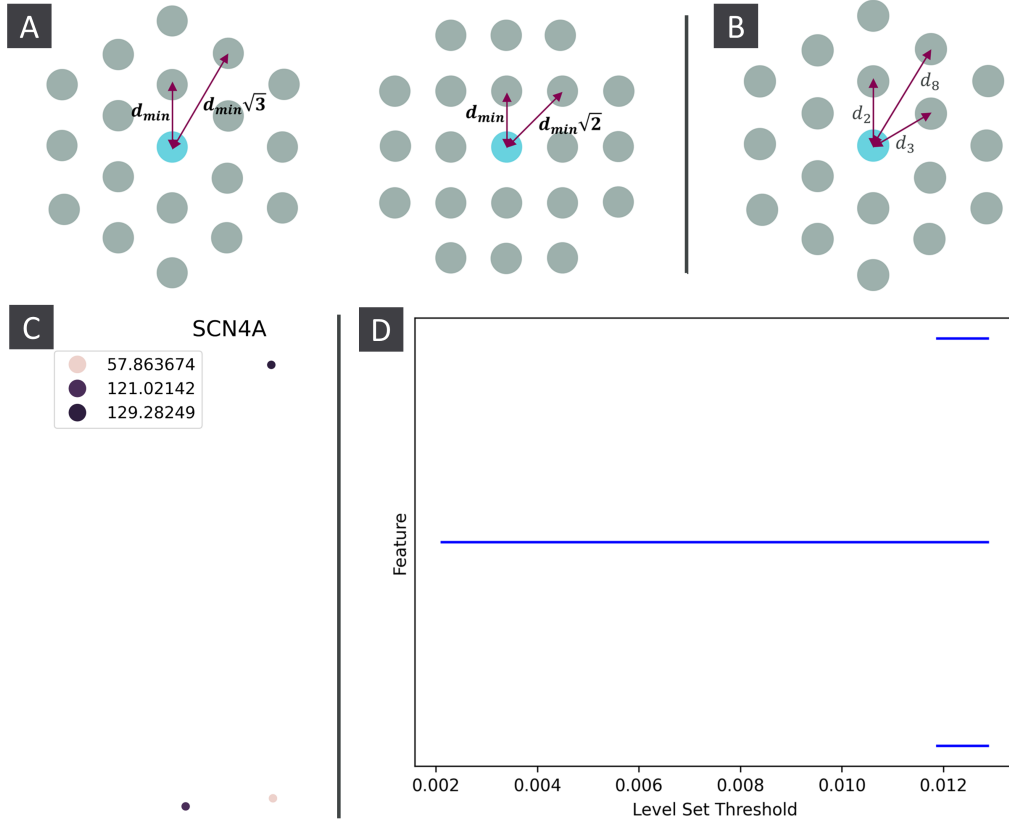

Supp Fig. 2: a,b) Illustration of how PersiST makes use of the wells lying on a regular grid structure - a) Distances between a central well (light blue) and its nearest and second nearest neighbours, in a hexagonal and square mesh. PersiST considers wells to be adjacent provided that they are separated by less than halfway between the minimum observed inter-well distance and the second nearest neighbour distance in a perfect grid where the minimum observed inter-well distance is the well separation. b) Figure illustrating the 2<sup>nd</sup>, 3<sup>rd</sup>, and 8<sup>th</sup> shortest distances between a central node (light blue) and the surrounding nodes (grey) in a hexagonal grid.  $d_1 = 0$ , as the distance from the light blue node to itself. c) Expression of SCN4A in kmp sample 30-10125 and d) the corresponding barcode diagram. The barcode is dominated by a single large bar, with a ratio of 0.91, so PersiST flags this as a possible artefact.

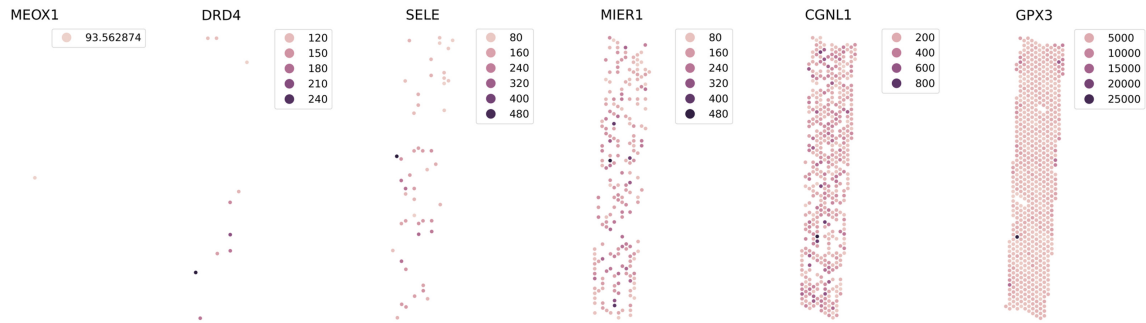

Supp Fig. 3: A selection of genes showing the range of variation in the number of wells in which each gene is expressed in sample 30-10125. Genes expressed in only a very small number of wells pose a challenge for SVG identification, as taken literally such patterns are extremely spatially significant (only being expressed in say two out of multiple hundred possible wells is in some sense very strong spatial localisation), but are not the kind of spatial structure practitioners typically have in mind when talking about Spatially Variable Genes.

## Supplementary Tables

|           | PersiST | Sepal  | SpatialDE | SPARK-X |
|-----------|---------|--------|-----------|---------|
| PersiST   | 1       | -0.003 | 0.302     | 0.159   |
| Sepal     | -0.003  | 1      | -0.001    | -0.003  |
| SpatialDE | 0.302   | -0.001 | 1         | 0.343   |
| SPARK-X   | 0.159   | -0.003 | 0.343     | 1       |

Supp Table 1: Adjusted Rand Index (ARI) for the different SVG identification methods applied to the kmp data set [13]. Values shown are mean average ARI across all samples.

|           | PersiST | Sepal | SpatialDE | SPARK-X |
|-----------|---------|-------|-----------|---------|
| PersiST   | 1       | 0     | 0.25      | 0.14    |
| Sepal     | 0       | 1     | 0.001     | 0.0001  |
| SpatialDE | 0.58    | 0.04  | 1         | 0.38    |
| SPARK-X   | 0.55    | 0.02  | 0.58      | 1       |

Supp Table 2: Overlap percentage for different SVG identification methods on the kmp data set [13]. The entry in row  $i$  column  $j$  is the percentage of genes called as SV by method  $j$  that method  $i$  also calls as SV, averaged across all the samples.

| method    | minimum | maximum | standard deviation | correlation with number of wells |
|-----------|---------|---------|--------------------|----------------------------------|
| PersiST   | 44      | 351     | 77.1               | 0.04                             |
| Sepal     | 0       | 491     | 133.1              | 0.66                             |
| SpatialDE | 662     | 15960   | 4475.0             | 0.34                             |
| SPARK-X   | 125     | 3918    | 1013.8             | 0.29                             |

Supp Table 3: Summary statistics for the number of SVGs called in each of the myocardial infarction samples [14], for each of the comparison methods. Correlations shown are Spearman correlation.

|           | PersiST | Sepal  | SpatialDE | SPARK-X |
|-----------|---------|--------|-----------|---------|
| PersiST   | 1       | -0.004 | 0.03      | 0.2     |
| Sepal     | -0.004  | 1      | 0.047     | -0.008  |
| SpatialDE | 0.03    | 0.047  | 1         | 0.117   |
| SPARK-X   | 0.2     | -0.008 | 0.117     | 1       |

Supp Table 4: Adjusted Rand Index (ARI) for the different SVG identification methods applied to the myocardial infarction data set [14]. Values shown are mean average ARI across all samples.

|           | PersiST | Sepal | SpatialDE | SPARK-X |
|-----------|---------|-------|-----------|---------|
| PersiST   | 1       | 0.004 | 0.04      | 0.16    |
| Sepal     | 0.003   | 1     | 0.008     | 0.001   |
| SpatialDE | 0.90    | 0.43  | 1         | 0.94    |
| SPARK-X   | 0.71    | 0.01  | 0.19      | 1       |

Supp Table 5: Overlap percentage for different SVG identification methods on the myocardial infarction data set [14]. The entry in row  $i$  column  $j$  is the average percentage of genes called as SV by method  $j$  that method  $i$  also calls as SV, averaged over all the samples.

## Further Supplementary Figures

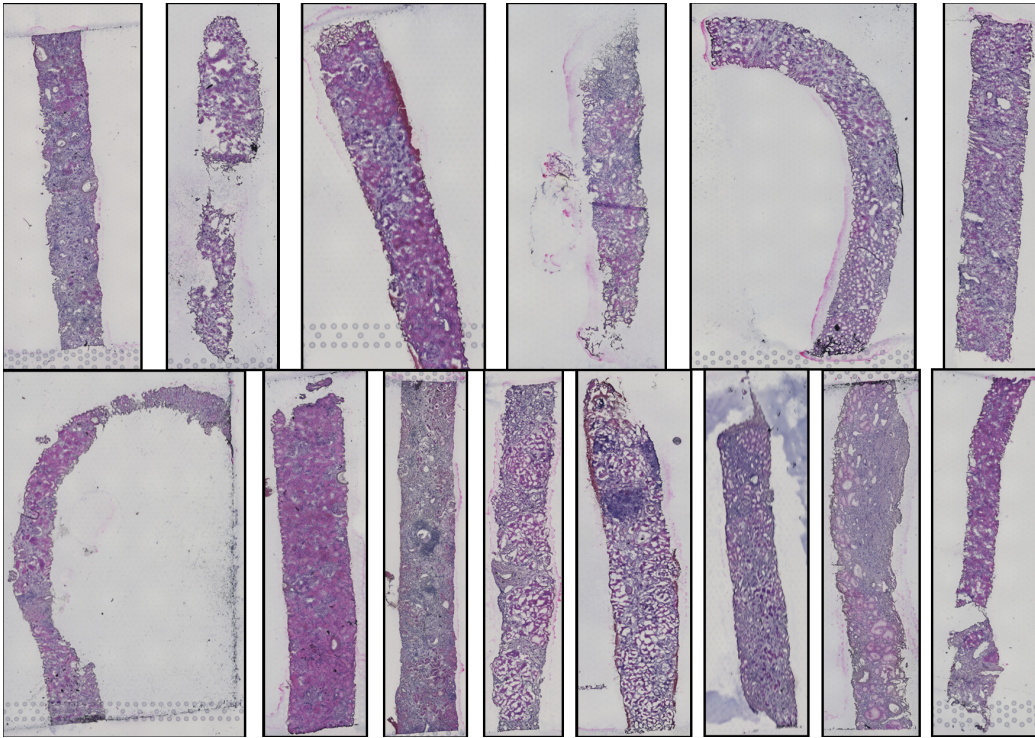

Supp Fig. 4: H&E Images for all analysed samples in the kpmp cohort [13]. The tissue slices display significant morphological variation.

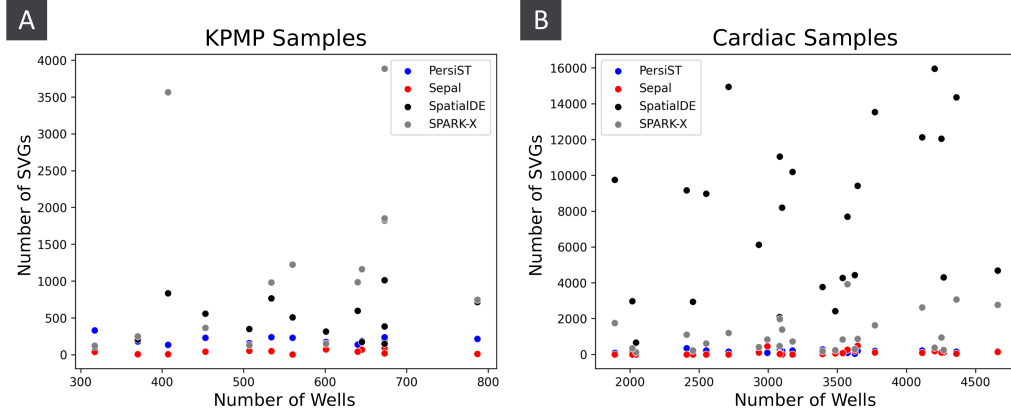

Supp Fig. 5: Plot of the number of SVGs identified by PersiST, SpatialDE, SPARK-X and Sepal against the number of wells for a) the kpmp samples and b) the cardiac samples.

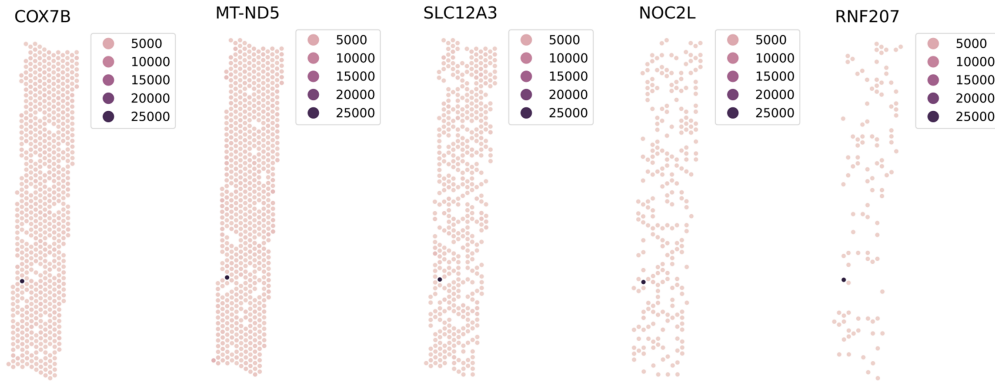

Supp Fig. 6: Co-expression of PersiST-SVGs COX7B, MT-ND5, SLC12A3, NOC2L, and RNF207 in kpmp sample 30-10135. The expression of all these genes is heavily localised to a single well.

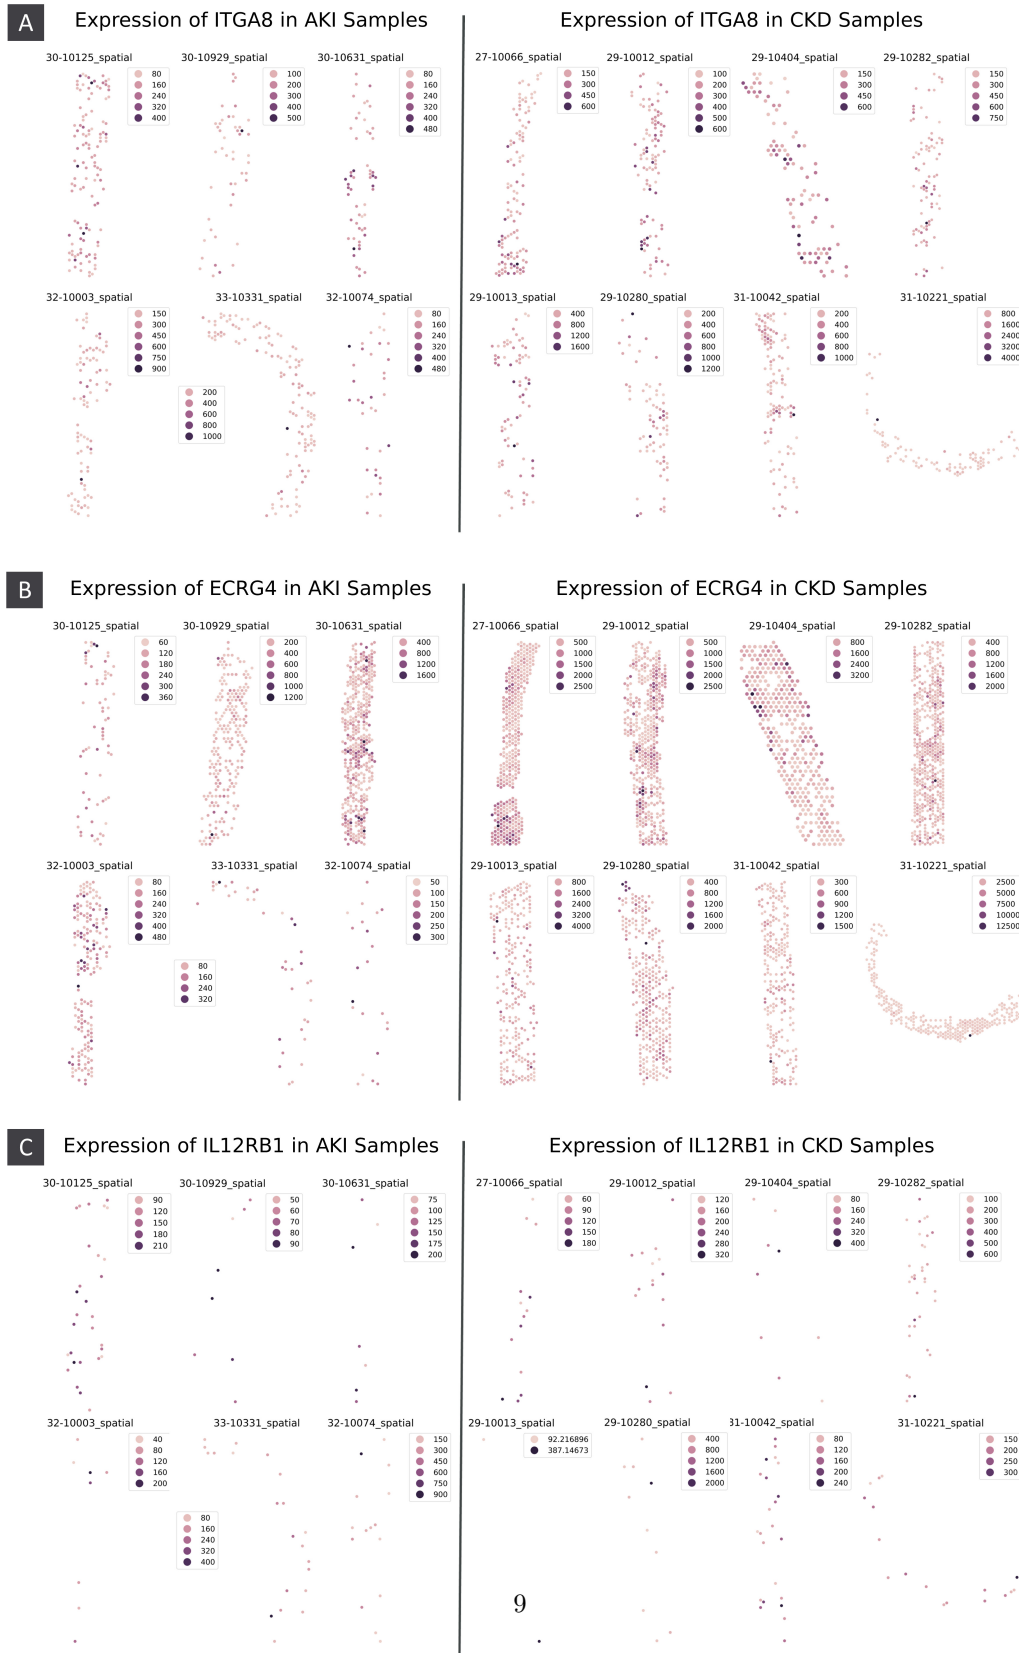

Supp Fig. 7: Expression of the genes with the highest difference in average a) SpatialDE computed adjusted q-value, b) SPARK-X computed q-value and c) sepal score between the AKI and CKD samples in the kpmp cohort.

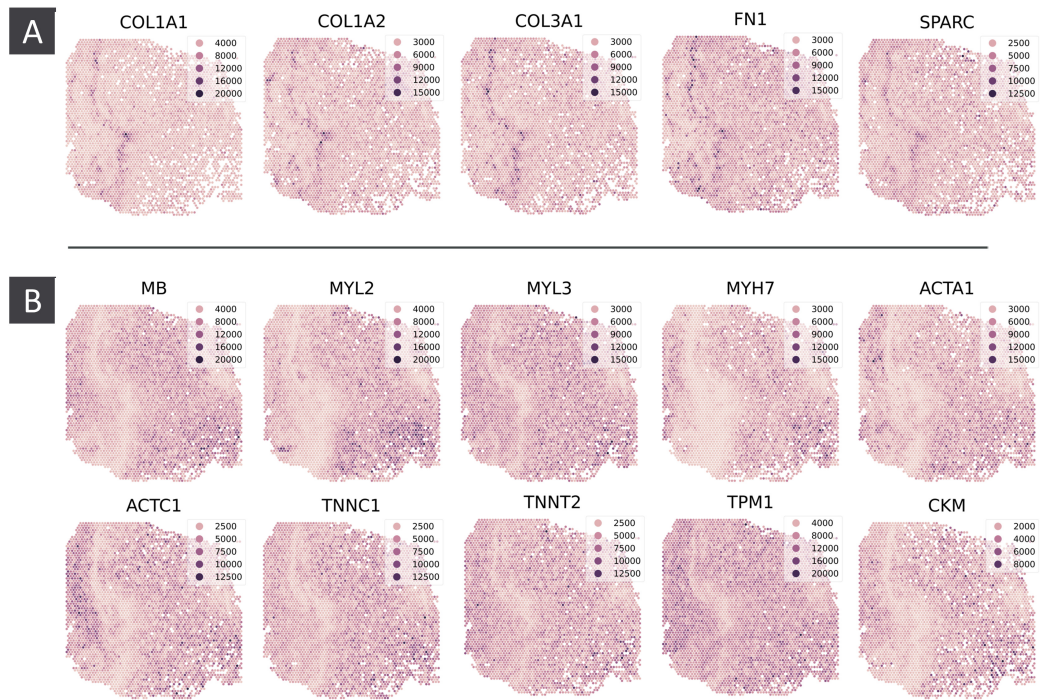

Supp Fig. 8: Full set of SVGs from figure 3. SVGs in figure a/b show elevated/lowered expression in the same region of the tissue.
